# Supplementary material for: Interpretation of multiple solutions in fully iterative GF2 and GW schemes using local analysis of two-particle density matrices
Source: arXiv:2104.12751 source file (2021-04-26)
Supplement: Supplementary file 1 [file SI.pdf]

# Interpretation of multiple solutions in fully iterative GF2 and GW schemes using local analysis of two-particle density matrices

Pavel Pokhilko[1] and Dominika Zgid[1,2]

[1]*Department of Chemistry, University of Michigan, Ann Arbor, Michigan 48109, USA*

[2]*Department of Physics, University of Michigan, Ann Arbor, Michigan 48109, USA*

## 1. FCI

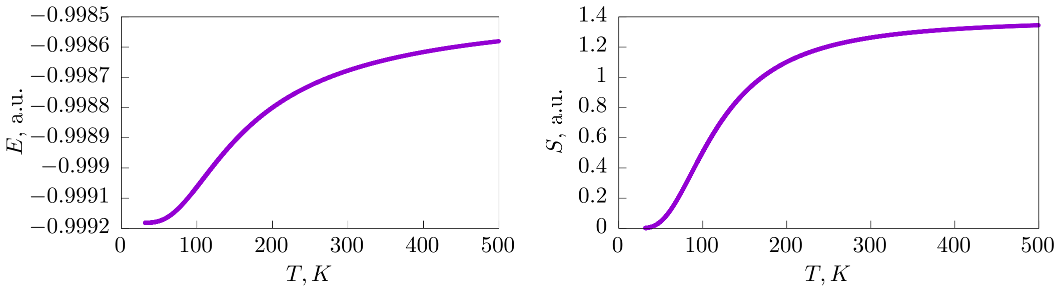


FIG. S1: The temperature dependence of the FCI ("exact diagonalization") internal energy and entropy for the $H_2$ molecule. Chemical potential was optimized at each temperature point to maintain the same number of electrons ($n = 2$). Smooth energy and entropy curves illustrate singlet-triplet transition. Symmetry breaking does not happen.

## 2. LOCAL SPIN AND CHARGE CORRELATORS FOR TRANSITION METAL COMPLEXES

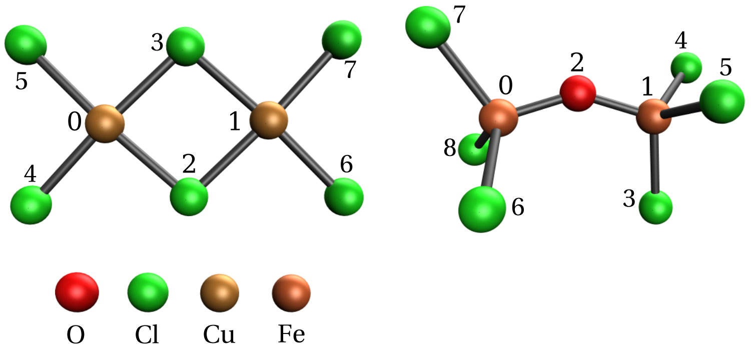


FIG. S2: The enumeration of atoms in the considered complexes (consistent with the ordering of lines in the provided Cartesian geometries).

TABLE S1: Differences in local spin correlators computed for $[Cu_2Cl_6]^{2-}$ with UHF ($\langle\vec{S}_A\vec{S}_B\rangle$(BS) - $\langle\vec{S}_A\vec{S}_B\rangle$(high spin)).

| $\Delta\langle\vec{S}_A\vec{S}_B\rangle$ | Cu(0) | Cu(1) | Cl(2) | Cl(3) | Cl(4) | Cl(5) | Cl(6) | Cl(7) |
|---|---|---|---|---|---|---|---|---|
| Cu(0) | $-1.7\cdot10^{-4}$ | $-0.42$ | $-0.029$ | $-0.029$ | $-7.0\cdot10^{-4}$ | $-7.0\cdot10^{-4}$ | $-0.034$ | $-0.034$ |
| Cu(1) | $-0.42$ | $-1.7\cdot10^{-4}$ | $-0.029$ | $-0.029$ | $-0.034$ | $-0.034$ | $-7.0\cdot10^{-4}$ | $-7.0\cdot10^{-4}$ |
| Cl(2) | $-0.029$ | $-0.029$ | $8.2\cdot10^{-3}$ | $-6.9\cdot10^{-3}$ | $-2.3\cdot10^{-3}$ | $-1.3\cdot10^{-3}$ | $-2.3\cdot10^{-3}$ | $-1.3\cdot10^{-3}$ |
| Cl(3) | $-0.029$ | $-0.029$ | $-6.9\cdot10^{-3}$ | $8.2\cdot10^{-3}$ | $-1.3\cdot10^{-3}$ | $-2.3\cdot10^{-3}$ | $-1.3\cdot10^{-3}$ | $-2.3\cdot10^{-3}$ |
| Cl(4) | $-7.0\cdot10^{-4}$ | $-0.034$ | $-2.3\cdot10^{-3}$ | $-1.3\cdot10^{-3}$ | $-4.1\cdot10^{-4}$ | $-7.8\cdot10^{-5}$ | $-2.7\cdot10^{-3}$ | $-2.7\cdot10^{-3}$ |
| Cl(5) | $-7.0\cdot10^{-4}$ | $-0.034$ | $-1.3\cdot10^{-3}$ | $-2.3\cdot10^{-3}$ | $-7.8\cdot10^{-5}$ | $-4.1\cdot10^{-4}$ | $-2.7\cdot10^{-3}$ | $-2.7\cdot10^{-3}$ |
| Cl(6) | $-0.034$ | $-7.0\cdot10^{-4}$ | $-2.3\cdot10^{-3}$ | $-1.3\cdot10^{-3}$ | $-2.7\cdot10^{-3}$ | $-2.7\cdot10^{-3}$ | $-4.1\cdot10^{-4}$ | $-7.8\cdot10^{-5}$ |
| Cl(7) | $-0.034$ | $-7.0\cdot10^{-4}$ | $-1.3\cdot10^{-3}$ | $-2.3\cdot10^{-3}$ | $-2.8\cdot10^{-3}$ | $-2.7\cdot10^{-3}$ | $-7.8\cdot10^{-5}$ | $-4.1\cdot10^{-4}$ |

TABLE S2: Differences in local spin correlators computed for $[Cu_2Cl_6]^{2-}$ with GW ($\langle\vec{S}_A\vec{S}_B\rangle$(BS) - $\langle\vec{S}_A\vec{S}_B\rangle$(high spin)).

| $\Delta\langle\vec{S}_A\vec{S}_B\rangle$ | Cu(0) | Cu(1) | Cl(2) | Cl(3) | Cl(4) | Cl(5) | Cl(6) | Cl(7) |
|---|---|---|---|---|---|---|---|---|
| Cu(0) | $-3.1\cdot10^{-3}$ | $-0.26$ | $-0.035$ | $-0.035$ | $-2.3\cdot10^{-3}$ | $-2.3\cdot10^{-3}$ | $-0.056$ | $-0.056$ |
| Cu(1) | $-0.26$ | $-3.1\cdot10^{-3}$ | $-0.035$ | $-0.035$ | $-0.056$ | $-0.056$ | $-2.3\cdot10^{-3}$ | $-2.3\cdot10^{-3}$ |
| Cl(2) | $-0.035$ | $-0.035$ | $0.042$ | $-0.028$ | $-7.4\cdot10^{-3}$ | $-5.6\cdot10^{-3}$ | $-7.3\cdot10^{-3}$ | $-5.6\cdot10^{-3}$ |
| Cl(3) | $-0.035$ | $-0.035$ | $-0.028$ | $0.042$ | $-5.6\cdot10^{-3}$ | $-7.3\cdot10^{-3}$ | $-5.6\cdot10^{-3}$ | $-7.3\cdot10^{-3}$ |
| Cl(4) | $-2.3\cdot10^{-3}$ | $-0.056$ | $-7.4\cdot10^{-3}$ | $-5.6\cdot10^{-3}$ | $-7.4\cdot10^{-3}$ | $-1.1\cdot10^{-3}$ | $-0.012$ | $-0.013$ |
| Cl(5) | $-2.3\cdot10^{-3}$ | $-0.056$ | $-5.5\cdot10^{-3}$ | $-7.4\cdot10^{-3}$ | $-1.1\cdot10^{-3}$ | $-7.4\cdot10^{-3}$ | $-0.013$ | $-0.012$ |
| Cl(6) | $-0.056$ | $-2.3\cdot10^{-3}$ | $-7.3\cdot10^{-3}$ | $-5.6\cdot10^{-3}$ | $-0.012$ | $-0.013$ | $-7.4\cdot10^{-3}$ | $-1.1\cdot10^{-3}$ |
| Cl(7) | $-0.056$ | $-2.3\cdot10^{-3}$ | $-5.6\cdot10^{-3}$ | $-7.3\cdot10^{-3}$ | $-0.013$ | $-0.012$ | $-1.1\cdot10^{-3}$ | $-7.4\cdot10^{-3}$ |

TABLE S3: Differences in local charge correlators computed for $[Cu_2Cl_6]^{2-}$ with UHF ($\langle\delta N_A\delta N_B\rangle$(BS) - $\langle\delta N_A\delta N_B\rangle$(high spin)).

| $\Delta\langle\delta N_A\delta N_B\rangle$ | Cu(0) | Cu(1) | Cl(2) | Cl(3) | Cl(4) | Cl(5) | Cl(6) | Cl(7) |
|---|---|---|---|---|---|---|---|---|
| Cu(0) | $-3.1\cdot10^{-4}$ | $2.8\cdot10^{-4}$ | $-3.1\cdot10^{-5}$ | $-3.1\cdot10^{-5}$ | $-1.0\cdot10^{-5}$ | $-1.0\cdot10^{-5}$ | $-4.5\cdot10^{-5}$ | $-4.5\cdot10^{-5}$ |
| Cu(1) | $2.8\cdot10^{-4}$ | $-3.1\cdot10^{-4}$ | $-3.1\cdot10^{-5}$ | $-3.1\cdot10^{-5}$ | $-4.5\cdot10^{-5}$ | $-4.5\cdot10^{-5}$ | $-1.0\cdot10^{-5}$ | $-1.0\cdot10^{-5}$ |
| Cl(2) | $-3.1\cdot10^{-5}$ | $-3.1\cdot10^{-5}$ | $-1.4\cdot10^{-4}$ | $-6.8\cdot10^{-4}$ | $-2.4\cdot10^{-5}$ | $3.1\cdot10^{-5}$ | $-2.4\cdot10^{-5}$ | $3.1\cdot10^{-5}$ |
| Cl(3) | $-3.1\cdot10^{-5}$ | $-3.1\cdot10^{-5}$ | $-6.8\cdot10^{-4}$ | $1.3\cdot10^{-4}$ | $3.1\cdot10^{-5}$ | $-2.4\cdot10^{-5}$ | $3.1\cdot10^{-5}$ | $-2.4\cdot10^{-5}$ |
| Cl(4) | $-1.0\cdot10^{-5}$ | $-4.5\cdot10^{-5}$ | $-2.4\cdot10^{-5}$ | $3.1\cdot10^{-5}$ | $3.4\cdot10^{-5}$ | $2.7\cdot10^{-5}$ | $4.0\cdot10^{-5}$ | $2.3\cdot10^{-5}$ |
| Cl(5) | $-1.0\cdot10^{-5}$ | $-4.5\cdot10^{-5}$ | $3.1\cdot10^{-5}$ | $-2.4\cdot10^{-5}$ | $2.7\cdot10^{-5}$ | $3.4\cdot10^{-5}$ | $2.3\cdot10^{-5}$ | $4.0\cdot10^{-5}$ |
| Cl(6) | $-4.5\cdot10^{-5}$ | $-1.0\cdot10^{-5}$ | $-2.4\cdot10^{-5}$ | $3.1\cdot10^{-5}$ | $4.0\cdot10^{-5}$ | $2.3\cdot10^{-5}$ | $3.3\cdot10^{-5}$ | $2.7\cdot10^{-5}$ |
| Cl(7) | $-4.5\cdot10^{-5}$ | $-1.0\cdot10^{-5}$ | $3.1\cdot10^{-5}$ | $-2.4\cdot10^{-5}$ | $2.3\cdot10^{-5}$ | $4.0\cdot10^{-5}$ | $2.7\cdot10^{-5}$ | $3.4\cdot10^{-5}$ |

TABLE S4: Differences in local charge correlators computed for $[Cu_2Cl_6]^{2-}$ with GW ($\langle \delta N_A \delta N_B \rangle$(BS) - $\langle \delta N_A \delta N_B \rangle$(high spin)).

| $\Delta \langle \delta N_A \delta N_B \rangle$ | Cu(0) | Cu(1) | Cl(2) | Cl(3) | Cl(4) | Cl(5) | Cl(6) | Cl(7) |
|---|---|---|---|---|---|---|---|---|
| Cu(0) | $-6.9 \cdot 10^{-5}$ | $6.8 \cdot 10^{-5}$ | $1.0 \cdot 10^{-4}$ | $1.0 \cdot 10^{-4}$ | $-1.8 \cdot 10^{-4}$ | $-1.8 \cdot 10^{-4}$ | $1.2 \cdot 10^{-4}$ | $1.2 \cdot 10^{-4}$ |
| Cu(1) | $6.8 \cdot 10^{-5}$ | $-6.9 \cdot 10^{-5}$ | $1.0 \cdot 10^{-4}$ | $1.0 \cdot 10^{-4}$ | $1.2 \cdot 10^{-4}$ | $1.2 \cdot 10^{-4}$ | $-1.8 \cdot 10^{-4}$ | $-1.8 \cdot 10^{-4}$ |
| Cl(2) | $1.0 \cdot 10^{-4}$ | $1.0 \cdot 10^{-4}$ | $-9.6 \cdot 10^{-4}$ | $-1.8 \cdot 10^{-3}$ | $3.7 \cdot 10^{-4}$ | $3.1 \cdot 10^{-4}$ | $3.7 \cdot 10^{-4}$ | $3.1 \cdot 10^{-4}$ |
| Cl(3) | $1.0 \cdot 10^{-4}$ | $1.0 \cdot 10^{-4}$ | $-1.8 \cdot 10^{-3}$ | $-9.6 \cdot 10^{-4}$ | $3.1 \cdot 10^{-4}$ | $3.7 \cdot 10^{-4}$ | $3.1 \cdot 10^{-4}$ | $3.7 \cdot 10^{-4}$ |
| Cl(4) | $-1.8 \cdot 10^{-4}$ | $1.2 \cdot 10^{-4}$ | $3.7 \cdot 10^{-4}$ | $3.1 \cdot 10^{-4}$ | $5.8 \cdot 10^{-5}$ | $-1.1 \cdot 10^{-5}$ | $-2.4 \cdot 10^{-4}$ | $3.2 \cdot 10^{-4}$ |
| Cl(5) | $-1.8 \cdot 10^{-4}$ | $1.1 \cdot 10^{-4}$ | $3.1 \cdot 10^{-4}$ | $3.7 \cdot 10^{-4}$ | $-1.1 \cdot 10^{-5}$ | $5.8 \cdot 10^{-5}$ | $3.2 \cdot 10^{-4}$ | $-2.4 \cdot 10^{-4}$ |
| Cl(6) | $1.2 \cdot 10^{-4}$ | $-1.8 \cdot 10^{-4}$ | $3.7 \cdot 10^{-4}$ | $3.1 \cdot 10^{-4}$ | $-2.4 \cdot 10^{-4}$ | $3.2 \cdot 10^{-4}$ | $5.8 \cdot 10^{-5}$ | $-1.1 \cdot 10^{-5}$ |
| Cl(7) | $1.2 \cdot 10^{-4}$ | $-1.8 \cdot 10^{-4}$ | $3.1 \cdot 10^{-4}$ | $3.7 \cdot 10^{-4}$ | $3.2 \cdot 10^{-4}$ | $-2.4 \cdot 10^{-4}$ | $-1.1 \cdot 10^{-5}$ | $5.8 \cdot 10^{-5}$ |

TABLE S5: Differences in local spin correlators computed for $[Fe_2OCl_6]^{2-}$ with UHF ($\langle \vec{S}_A \vec{S}_B \rangle$(BS) - $\langle \vec{S}_A \vec{S}_B \rangle$(high spin)).

| $\Delta \langle \vec{S}_A \vec{S}_B \rangle$ | Fe(0) | Fe(1) | O(2) | Cl(3) | Cl(4) | Cl(5) | Cl(6) | Cl(7) | Cl(8) |
|---|---|---|---|---|---|---|---|---|---|
| Fe(0) | $2.2 \cdot 10^{-3}$ | $-11.6$ | $-0.67$ | $-0.33$ | $-0.32$ | $-0.34$ | $6.6 \cdot 10^{-3}$ | $-0.013$ | $-0.003$ |
| Fe(1) | $-11.6$ | $2.2 \cdot 10^{-3}$ | $-0.67$ | $6.6 \cdot 10^{-3}$ | $-0.013$ | $-3.4 \cdot 10^{-3}$ | $-0.33$ | $-0.32$ | $-0.33$ |
| O(2) | $-0.67$ | $-0.67$ | $-0.15$ | $-0.017$ | $-0.016$ | $-0.019$ | $-0.017$ | $-0.016$ | $-0.019$ |
| Cl(3) | $-0.33$ | $6.6 \cdot 10^{-3}$ | $-0.017$ | $3.4 \cdot 10^{-3}$ | $4.8 \cdot 10^{-4}$ | $2.8 \cdot 10^{-4}$ | $-0.010$ | $-0.012$ | $-0.010$ |
| Cl(4) | $-0.32$ | $-0.013$ | $-0.016$ | $4.8 \cdot 10^{-4}$ | $-0.013$ | $6.7 \cdot 10^{-4}$ | $-0.012$ | $-8.0 \cdot 10^{-3}$ | $-7.5 \cdot 10^{-3}$ |
| Cl(5) | $-0.33$ | $-3.4 \cdot 10^{-3}$ | $-0.019$ | $2.8 \cdot 10^{-4}$ | $6.7 \cdot 10^{-4}$ | $-3.8 \cdot 10^{-3}$ | $-9.9 \cdot 10^{-3}$ | $-7.4 \cdot 10^{-3}$ | $-0.013$ |
| Cl(6) | $6.6 \cdot 10^{-3}$ | $-0.33$ | $-0.017$ | $-0.010$ | $-0.012$ | $-0.010$ | $3.4 \cdot 10^{-3}$ | $4.8 \cdot 10^{-4}$ | $2.8 \cdot 10^{-4}$ |
| Cl(7) | $-0.013$ | $-0.32$ | $-0.016$ | $-0.012$ | $-8.0 \cdot 10^{-3}$ | $-7.5 \cdot 10^{-3}$ | $4.8 \cdot 10^{-4}$ | $-0.013$ | $6.7 \cdot 10^{-4}$ |
| Cl(8) | $-3.4 \cdot 10^{-3}$ | $-0.33$ | $-0.019$ | $-0.010$ | $-7.5 \cdot 10^{-3}$ | $-0.013$ | $2.8 \cdot 10^{-4}$ | $6.7 \cdot 10^{-4}$ | $-3.8 \cdot 10^{-3}$ |

TABLE S6: Differences in local spin correlators computed for $[Fe_2OCl_6]^{2-}$ with GW ($\langle \vec{S}_A \vec{S}_B \rangle$(BS) - $\langle \vec{S}_A \vec{S}_B \rangle$(high spin)).

| $\Delta \langle \vec{S}_A \vec{S}_B \rangle$ | Fe(0) | Fe(1) | O(2) | Cl(3) | Cl(4) | Cl(5) | Cl(6) | Cl(7) | Cl(8) |
|---|---|---|---|---|---|---|---|---|---|
| Fe(0) | $0.16$ | $-10.0$ | $-0.79$ | $-0.50$ | $-0.49$ | $-0.49$ | $-0.014$ | $-0.049$ | $-0.031$ |
| Fe(1) | $-10.0$ | $0.16$ | $-0.79$ | $-0.014$ | $-0.049$ | $-0.031$ | $-0.50$ | $-0.49$ | $-0.49$ |
| O(2) | $-0.79$ | $-0.79$ | $-0.27$ | $-0.039$ | $-0.032$ | $-0.040$ | $-0.039$ | $-0.032$ | $-0.040$ |
| Cl(3) | $-0.50$ | $-0.014$ | $-0.039$ | $-0.017$ | $-4.9 \cdot 10^{-4}$ | $-4.4 \cdot 10^{-4}$ | $-0.027$ | $-0.033$ | $-0.026$ |
| Cl(4) | $-0.49$ | $-0.049$ | $-0.032$ | $-4.9 \cdot 10^{-4}$ | $-0.050$ | $-7.8 \cdot 10^{-4}$ | $-0.033$ | $-0.020$ | $-0.020$ |
| Cl(5) | $-0.49$ | $-0.031$ | $-0.040$ | $-4.4 \cdot 10^{-4}$ | $-7.8 \cdot 10^{-4}$ | $-0.035$ | $-0.026$ | $-0.020$ | $-0.035$ |
| Cl(6) | $-0.014$ | $-0.50$ | $-0.039$ | $-0.027$ | $-0.033$ | $-0.026$ | $-0.017$ | $-5.0 \cdot 10^{-4}$ | $-4.4 \cdot 10^{-4}$ |
| Cl(7) | $-0.049$ | $-0.49$ | $-0.032$ | $-0.033$ | $-0.020$ | $-0.020$ | $-5.0 \cdot 10^{-4}$ | $-0.050$ | $-7.8 \cdot 10^{-4}$ |
| Cl(8) | $-0.031$ | $-0.49$ | $-0.040$ | $-0.026$ | $-0.020$ | $-0.035$ | $-4.4 \cdot 10^{-4}$ | $-7.8 \cdot 10^{-4}$ | $-0.035$ |

TABLE S7: Differences in local spin correlators computed for $[Fe_2OCl_6]^{2-}$ with UHF ($\langle \delta N_A \delta N_B \rangle$(BS) - $\langle \delta N_A \delta N_B \rangle$(high spin)).

| | Fe(0) | Fe(1) | O(2) | Cl(3) | Cl(4) | Cl(5) | Cl(6) | Cl(7) | Cl(8) |
|---|---|---|---|---|---|---|---|---|---|
| Fe(0) | $4.3 \cdot 10^{-3}$ | $-2.6 \cdot 10^{-3}$ | $-3.1 \cdot 10^{-3}$ | $-4.1 \cdot 10^{-4}$ | $1.3 \cdot 10^{-4}$ | $-3.7 \cdot 10^{-5}$ | $3.1 \cdot 10^{-4}$ | $1.4 \cdot 10^{-4}$ | $2.0 \cdot 10^{-4}$ |
| Fe(1) | $-2.6 \cdot 10^{-3}$ | $4.3 \cdot 10^{-3}$ | $-3.1 \cdot 10^{-3}$ | $3.1 \cdot 10^{-4}$ | $1.4 \cdot 10^{-4}$ | $2.0 \cdot 10^{-4}$ | $-4.1 \cdot 10^{-4}$ | $1.3 \cdot 10^{-4}$ | $-3.7 \cdot 10^{-5}$ |
| O(2) | $-3.1 \cdot 10^{-3}$ | $-3.1 \cdot 10^{-3}$ | 0.040 | $2.5 \cdot 10^{-4}$ | $8.9 \cdot 10^{-4}$ | $6.0 \cdot 10^{-4}$ | $2.5 \cdot 10^{-4}$ | $8.9 \cdot 10^{-4}$ | $6.0 \cdot 10^{-4}$ |
| Cl(3) | $-4.1 \cdot 10^{-4}$ | $3.1 \cdot 10^{-4}$ | $2.5 \cdot 10^{-4}$ | $-3.9 \cdot 10^{-4}$ | $-3.2 \cdot 10^{-5}$ | $1.3 \cdot 10^{-5}$ | $1.1 \cdot 10^{-4}$ | $9.8 \cdot 10^{-5}$ | $2.7 \cdot 10^{-5}$ |
| Cl(4) | $1.3 \cdot 10^{-4}$ | $1.4 \cdot 10^{-4}$ | $8.9 \cdot 10^{-4}$ | $-3.2 \cdot 10^{-5}$ | $5.5 \cdot 10^{-4}$ | $-1.4 \cdot 10^{-4}$ | $9.8 \cdot 10^{-5}$ | $1.0 \cdot 10^{-4}$ | $2.3 \cdot 10^{-6}$ |
| Cl(5) | $-3.7 \cdot 10^{-5}$ | $2.0 \cdot 10^{-4}$ | $6.0 \cdot 10^{-4}$ | $1.3 \cdot 10^{-5}$ | $-1.4 \cdot 10^{-4}$ | $1.1 \cdot 10^{-4}$ | $2.7 \cdot 10^{-5}$ | $2.3 \cdot 10^{-6}$ | $1.6 \cdot 10^{-4}$ |
| Cl(6) | $3.1 \cdot 10^{-4}$ | $-4.1 \cdot 10^{-4}$ | $2.5 \cdot 10^{-4}$ | $1.2 \cdot 10^{-4}$ | $9.8 \cdot 10^{-5}$ | $2.7 \cdot 10^{-5}$ | $-3.9 \cdot 10^{-4}$ | $-3.2 \cdot 10^{-5}$ | $1.3 \cdot 10^{-5}$ |
| Cl(7) | $1.4 \cdot 10^{-4}$ | $1.3 \cdot 10^{-4}$ | $8.9 \cdot 10^{-4}$ | $9.8 \cdot 10^{-5}$ | $1.0 \cdot 10^{-4}$ | $2.3 \cdot 10^{-6}$ | $-3.2 \cdot 10^{-5}$ | $5.5 \cdot 10^{-4}$ | $-1.4 \cdot 10^{-4}$ |
| Cl(8) | $2.0 \cdot 10^{-4}$ | $-3.7 \cdot 10^{-5}$ | $6.0 \cdot 10^{-4}$ | $2.7 \cdot 10^{-5}$ | $2.3 \cdot 10^{-6}$ | $1.6 \cdot 10^{-4}$ | $1.3 \cdot 10^{-5}$ | $-1.4 \cdot 10^{-4}$ | $1.1 \cdot 10^{-4}$ |

TABLE S8: Differences in local spin correlators computed for $[Fe_2OCl_6]^{2-}$ with GW ($\langle \delta N_A \delta N_B \rangle$(BS) - $\langle \delta N_A \delta N_B \rangle$(high spin)).

| | Fe(0) | Fe(1) | O(2) | Cl(3) | Cl(4) | Cl(5) | Cl(6) | Cl(7) | Cl(8) |
|---|---|---|---|---|---|---|---|---|---|
| Fe(0) | 0.032 | $-0.011$ | $-1.9 \cdot 10^{-3}$ | $-1.1 \cdot 10^{-3}$ | $-6.3 \cdot 10^{-4}$ | $-9.6 \cdot 10^{-4}$ | $3.0 \cdot 10^{-3}$ | $2.2 \cdot 10^{-3}$ | $2.8 \cdot 10^{-3}$ |
| Fe(1) | $-0.011$ | 0.032 | $-1.9 \cdot 10^{-3}$ | $3.0 \cdot 10^{-3}$ | $2.2 \cdot 10^{-3}$ | $2.8 \cdot 10^{-3}$ | $-1.1 \cdot 10^{-3}$ | $-6.3 \cdot 10^{-4}$ | $-9.6 \cdot 10^{-4}$ |
| O(2) | $-1.9 \cdot 10^{-3}$ | $-1.9 \cdot 10^{-3}$ | 0.049 | $2.5 \cdot 10^{-3}$ | $2.3 \cdot 10^{-3}$ | $2.6 \cdot 10^{-3}$ | $2.5 \cdot 10^{-3}$ | $2.3 \cdot 10^{-3}$ | $2.6 \cdot 10^{-3}$ |
| Cl(3) | $-1.1 \cdot 10^{-3}$ | $3.0 \cdot 10^{-3}$ | $2.5 \cdot 10^{-3}$ | $8.2 \cdot 10^{-4}$ | $2.1 \cdot 10^{-4}$ | $1.7 \cdot 10^{-4}$ | $-1.7 \cdot 10^{-4}$ | $-1.7 \cdot 10^{-4}$ | $-1.4 \cdot 10^{-4}$ |
| Cl(4) | $-6.3 \cdot 10^{-4}$ | $2.2 \cdot 10^{-3}$ | $2.3 \cdot 10^{-3}$ | $2.1 \cdot 10^{-4}$ | $1.8 \cdot 10^{-3}$ | $1.8 \cdot 10^{-4}$ | $-1.7 \cdot 10^{-4}$ | $-2.6 \cdot 10^{-4}$ | $-2.6 \cdot 10^{-4}$ |
| Cl(5) | $-9.6 \cdot 10^{-4}$ | $2.8 \cdot 10^{-3}$ | $2.6 \cdot 10^{-3}$ | $1.7 \cdot 10^{-4}$ | $1.8 \cdot 10^{-4}$ | $1.3 \cdot 10^{-3}$ | $-1.4 \cdot 10^{-4}$ | $-2.6 \cdot 10^{-4}$ | $-2.7 \cdot 10^{-4}$ |
| Cl(6) | $3.0 \cdot 10^{-3}$ | $-1.1 \cdot 10^{-3}$ | $2.5 \cdot 10^{-3}$ | $-1.7 \cdot 10^{-4}$ | $-1.7 \cdot 10^{-4}$ | $-1.4 \cdot 10^{-4}$ | $8.2 \cdot 10^{-4}$ | $2.1 \cdot 10^{-4}$ | $1.7 \cdot 10^{-4}$ |
| Cl(7) | $2.2 \cdot 10^{-3}$ | $-6.3 \cdot 10^{-4}$ | $2.3 \cdot 10^{-3}$ | $-1.7 \cdot 10^{-4}$ | $-2.6 \cdot 10^{-4}$ | $-2.6 \cdot 10^{-4}$ | $2.1 \cdot 10^{-4}$ | $1.8 \cdot 10^{-3}$ | $1.8 \cdot 10^{-4}$ |
| Cl(8) | $2.8 \cdot 10^{-3}$ | $-9.6 \cdot 10^{-4}$ | $2.6 \cdot 10^{-3}$ | $-1.4 \cdot 10^{-4}$ | $-2.6 \cdot 10^{-4}$ | $-2.7 \cdot 10^{-4}$ | $1.7 \cdot 10^{-4}$ | $1.8 \cdot 10^{-4}$ | $1.3 \cdot 10^{-3}$ |

## 3. CARTESIAN GEOMETRIES

$H_2$ molecule

```
H 0.00 0.00 -1.575
H 0.00 0.00  1.575
```

$H_4$ molecule

```
H  1.11369318  1.11369318  1.11369318
H  1.11369318 -1.11369318 -1.11369318
H -1.11369318  1.11369318 -1.11369318
H -1.11369318 -1.11369318  1.11369318
```

$Cu_2Cl_6^{2-}$ complex

```
Cu      -0.44198447       1.04236051      -0.03573258
Cu       2.94244268       1.24888730       0.03573258
Cl       1.34164711      -0.39956189       0.13607601
Cl       1.15881110       2.69080969      -0.13607601
Cl      -1.89798505      -0.68257133       0.07504862
Cl      -2.09088015       2.57782327      -0.21207639
Cl       4.59133836      -0.28657547       0.21207639
Cl       4.39844326       2.97381913      -0.07504862
```

$Fe_2OCl_6^{2-}$ complex

```
 Fe     0.0000000     0.0000000     0.0000000
 Fe     1.0206400    -0.0000000     3.1966814
 O     -0.0000000     0.0000000     1.7612762
 Cl     2.9139281     1.0985926     2.7935616
 Cl    -0.0643060     0.9830549     4.8598356
 Cl     1.4870706    -2.0787841     3.7767564
 Cl     1.7766011    -1.0984941    -0.7685878
 Cl    -1.8479834    -0.9829565    -0.7267066
 Cl     0.0439901     2.0788825    -0.7430241
```
